# Supplementary material for: A Graph Neural Network Approach to Automated Model Building in Cryo-EM Maps
Source: arXiv:2210.00006 source file (2023-02-08)
Supplement: Supplementary file 1 [file symbols.tex]

\subsection{Symbols}
    \centerline{\bf Symbol Names}
    \bgroup
    
    \begin{tabular}{p{1in}p{3.25in}}
    $\displaystyle N$ & Number of residues/nodes \\
    $\displaystyle d$ & Dimension of feature vectors \\
    $\displaystyle v$ & Box size of the cryo-EM map \\
    $\displaystyle k$ & Number of neighbours, default set to 20 \\
    $\displaystyle p$ & Number of query points per node, default set to 4 \\
    $\displaystyle \mV$ & cryo-EM map, $\R^{v \times v \times v}$\\
    $\displaystyle \caPos$ & $\calpha$ positions, $\R^{N \times 3}$\\
    $\displaystyle \mathbf{z}$ & Node features, $\R^{N \times d}$\\
    $\displaystyle \mathbf{F}$ & Backbone frames, $\R^{N \times 3 \times 4}$\\
    $\displaystyle [\cdot, \cdot]$ & Concatenation, $\R^{\cdots a}, \R^{\cdots b} \rightarrow \R^{\cdots a + b}$ \\
    \end{tabular}
    \egroup
    \vspace{0.25cm}
